# Supplementary material for: Mid-circuit cavity measurement in a neutral atom array
Source: arXiv:2205.14138 source file (2022-10-07)
Supplement: Supplementary file 1 [file supplement.pdf]

# Supplemental Material:
# Mid-circuit cavity measurement in a neutral atom array

Emma Deist,[1,2,*] Yue-Hui Lu,[1,2,*] Jacquelyn Ho,[1,2] Mary Kate Pasha,[1,2]
Johannes Zeiher,[1,3,4] Zhenjie Yan,[1,2] and Dan M. Stamper-Kurn[1,2,5,†]

[1]*Department of Physics, University of California, Berkeley, California 94720*
[2]*Challenge Institute for Quantum Computation, University of California, Berkeley, California 94720*
[3]*Max-Planck-Institut für Quantenoptik, 85748 Garching, Germany*
[4]*Munich Center for Quantum Science and Technology (MCQST), 80799 Munich, Germany*
[5]*Materials Sciences Division, Lawrence Berkeley National Laboratory, Berkeley, California 94720*

## ATOM PREPARATION AND STATE INITIALIZATION

Our optical tweezer array is formed by multiple beams of light at a wavelength of 808 nm generated by an acousto-optic deflector (AOD). The tweezer beams are focused through a NA = 0.5 objective to a beam waist radius ($1/e^2$ intensity) of 750 nm. The tweezer array is initially overlapped with an optical dipole trap at a wavelength of 1064 nm, containing a non-degenerate gas of $10^5$ $^{87}$Rb atoms with a temperature of 30 $\mu$K and $1/e$ density radius of 10 $\mu$m (2 mm) along its radial (axial) direction. The dipole trap is extinguished 10 ms after switching on the tweezer traps. The tweezers are then exposed to one-dimensional polarization gradient cooling (PGC) light and repump light for 125 ms, reducing the atom number in each tweezer to either zero or one [S1], while the atomic fluorescence is collected through the high-NA objective (exposure time of 100 ms) to determine the tweezer occupation. While we estimate a radial density width of 200 nm in the tweezers after 1D PGC [S2], we expect a reduction to below 100 nm with 3D PGC [S3] or around 50 nm with Raman sideband cooling [S4].

After tweezer loading and imaging, the atoms are prepared in the $F = 1$ and $F = 2$ ground state manifolds without Zeeman-state-specificity for the cavity measurements shown in Figs. 2 and 3. For initialization in the $F = 1$ ($F = 2$) manifold, the atoms are exposed to depump (repump) light resonant with the $D_2$ $F = 2$ ($F = 1$)$\rightarrow F' = 2$ transition for 0.75 ms (2 ms).

For the mid-circuit measurement sequence shown in Fig. 4, the atoms are prepared in the initial state $|F = 2, m_F = 0\rangle$. Under an applied bias magnetic field of 5 G, we illuminate the atoms simultaneously with $\pi$-polarized depump light and $\sigma^{\pm}$-polarized repump light for 1 ms. This optical pumping process results in a 90% preparation fidelity based on the contrast of Rabi oscillations observed immediately after state preparation on the $|F = 2, m_F = 0\rangle \rightarrow |F = 1, m_F = 0\rangle$ microwave transition.

## CAVITY PARAMETERS

Cavity ringdown measurements yield a cavity half width at half maximum of $\kappa = 2\pi \times 0.53$ MHz and a finesse of 14700 for the cavity mode at 780 nm wavelength [S5]. Using single atom scanning probe microscopy, we measured the cavity mode waist radius ($1/e^2$ intensity) to be $w_0 = 20(3)$ $\mu$m [S2]. With a cavity length of 9.4 mm, we derive the maximum atom-cavity coupling strength for the $|F = 2, m_F = 2\rangle \rightarrow |F = 3, m_F = 3\rangle$ stretched state transition to be $g_0 = 2\pi \times 2.7$ MHz.

To facilitate detection, the optical cavity features two mirrors with asymmetric transmissivity of 3.5 and 250 ppm at the probe wavelength of 780 nm. With total loss and transmission of 430 ppm based on the measured cavity finesse, cavity photons thus enter the detection optics through the cavity's more transmissive outcoupling mirror with an efficiency of 58%. These photons are routed into an optical fiber and onto a single photon counting module (SPCM: SPCM-AQR-13) with total optical path efficiency of 65%. The quantum efficiency of the detector is 66%. Multiplying these three factors yields an overall cavity photon detection efficiency of $\eta = 25\%$.

The cavity length is tuned and stabilized by driving the cavity with narrow and tunable frequency light at a wavelength of 1560 nm, and locking the cavity so that this light is resonant with a $\mathrm{TEM}_{01}$ cavity mode. The dark plane of this $\mathrm{TEM}_{01}$ mode is horizontal. The vertical height of the tweezer array is tuned so that atoms are trapped and also translated horizontally along this dark plane, minimizing their exposure to 1560-nm-wavelength light. In this manner, ac Stark shifts on the $D_2$ transition that would be produced by the cavity-locking light (as measured previously in Ref. [S2]) are eliminated.

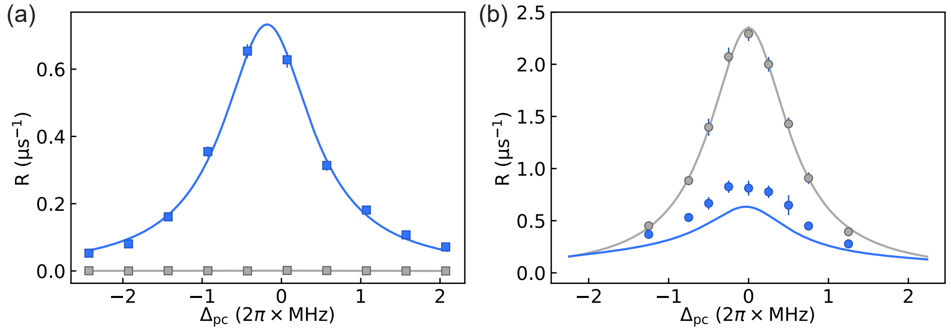


Figure S1. Cavity fluorescence and transmission spectrum. (a) Fluorescence photodetection rate vs. $\Delta_{\mathrm{pc}}$. A Lorentzian lineshape is fitted for the bright state fluorescence $R_{\mathrm{high}}$ (blue points). The Lorentzian fit (blue line) yields a half-linewidth of $2\pi \times 0.68(3)$ MHz; the center of the peak is shifted from bare cavity resonance by $2\pi \times -0.15(2)$ MHz because of the atom-induced ac Stark shift. $R_{\mathrm{low}}$ (gray) is measured with no atom trapped in the cavity. (b) Transmission photodetection rates vs. $\Delta_{\mathrm{pc}}$. $R_{\mathrm{high}}$ (gray points) exhibit a Lorentzian lineshape (gray curve) with fitted half-linewidth of $2\pi \times 0.60(2)$ MHz, slightly larger than $\kappa$ (measured by cavity ringdown). For these calibration data, $R_{\mathrm{low}}$ (blue points) is reduced to $0.35 \times R_{\mathrm{high}}$ on resonance (slightly different than for the measurements reported in the main text). Its variation with $\Delta_{\mathrm{pc}}$ agrees qualitatively with theoretical prediction based on the Jaynes-Cummings model and including effects of spatial averaging of $g^2$ along the cavity axis (blue curve). The fact that $R_{\mathrm{low}}$ is overall higher than expected based on this theoretical prediction may be explained by ac Stark shifts of the atomic resonance line by tweezer light. Error bars in (a) and (b) indicate the standard errors in the mean photon detection rate determined from repeated measurements.

## CAVITY FLUORESCENCE AND TRANSMISSION

In Fig. S1, we show the cavity photon detection rate for the fluorescence and transmission methods of detection, with the probe frequency and intensity settings described in the main text, and with variable cavity resonance frequency (indicated by $\Delta_{\mathrm{pc}}$). As described in the main text, with $\Delta_{\mathrm{pc}}$ near zero, we observe a large difference between the detection rates observed with an $F = 2$ atom in the cavity (blue points) and those observed with no atom in the cavity (gray points).

The observed rates can be matched with theoretical predictions. We consider a simple model in which our system can be described by the Jaynes-Cummings Hamiltonian, with additional atomic and cavity driving terms describing the fluorescence and transmission probe light, as well as cavity photon decay at a rate $2\kappa$ and atomic excited state population decay at a rate $2\gamma$. The atom is treated as a two-level system (operated upon by the standard $\hat{\sigma}$ operators), ignoring significant dynamics of the atom within its hyperfine structure. Further, the cavity is treated as a single-mode system, ignoring the existence of two near-degenerate cavity modes of opposite polarization. In the steady state, the rate of detecting cavity photons is $R = 2\eta\kappa\langle\hat{a}^\dagger\hat{a}\rangle$, with $\hat{a}$ being the cavity mode annihilation operator.

Considering first the fluorescence measurement, we adopt a mean-field approximation, replacing terms like $\langle\hat{a}\hat{\sigma}^+\rangle$ with $\langle\hat{a}\rangle\langle\hat{\sigma}^+\rangle$. This yields a steady-state photon field $\langle\hat{a}\rangle = ig_0\langle\hat{\sigma}^-\rangle/(\kappa - i\Delta_{\mathrm{pc}})$ and a photon detection rate $R = 2\eta\kappa\langle\hat{a}\rangle^2 = 2\eta\kappa {g_0}^2\langle\hat{\sigma}^-\rangle^2/(\kappa^2 + {\Delta_{\mathrm{pc}}}^2)$. At $\Delta_{\mathrm{pc}} = 0$, a maximum cavity detection rate of $R_0 = \eta\, g_0^2/(4\kappa)$ is expected when $\langle\hat{\sigma}^-\rangle^2$ reaches its maximum value of 1/8. This result agrees well with the maximum cavity scattering observed in numerical simulation of the Jaynes-Cummings master equation that we perform using QuTiP [S6]. In Fig. S1(a), we show the detected photon counts vs. $\Delta_{\mathrm{pc}}$ fitted to a Lorentzian, which has a half-linewidth slightly larger than $\kappa$; this extra broadening may be caused by noise in $\Delta_{\mathrm{pc}}$ and cavity quantum electrodynamic effects.

The observed maximum cavity emission rate is not captured by the mean-field model of a two-level atom and single cavity mode. Numerical calculation of the cavity photodetection rate $R_{\parallel,\mathrm{eff}}$ ($R_{\perp,\mathrm{eff}}$) under probe light polarized along (perpendicular to) the cavity axis yields $R_{\parallel,\mathrm{eff}} = 0.10R_{\mathrm{max}}$ ($R_{\perp,\mathrm{eff}} = 0.50R_{\mathrm{max}}$). The fluorescence probe beams are in a lin-perp-lin molasses configuration that alternates between these two polarizations. Spatial averaging of the probe polarization and equal population of the Zeeman sublevels result in a reduction of the theoretical $R_{\mathrm{max}}$ by a factor of 0.28.

Next we move to the transmission measurements, where the two-level picture is more applicable because the atom is pumped to the stretched state by the circularly polarized transmission probe light. Fig. S1(b) shows the transmission through the cavity versus $\Delta_{\mathrm{pc}}$ in the low-saturation regime. The theoretical factor of $R_{\mathrm{low}}/R_{\mathrm{high}}$ vs. $\Delta_{\mathrm{pc}}$ in the weak-drive regime is given in Ref. [S7]. Taking that result, and performing a uniform spatial average along the cavity axis, we obtain the blue curve shown in Fig. S1(b). Both this predicted and the observed $R_{\mathrm{low}}$ transmission line shape are broadened with respect to that of the empty cavity. The observed cavity transmission $R_{\mathrm{low}}$ is generally higher

than the predicted value. This discrepancy is likely caused by ac Stark shift variation produced by the optical tweezer light.

In Fig. 3(c), we use Ashman's $D$ function [S8] to quantify the separation of the high and low cavity transmission distributions. Considering two distributions with means $\mu_{1,2}$ and standard deviations $\sigma_{1,2}$, Ashman's $D$ is defined as $D = |\mu_1 - \mu_2|/\sqrt{(\sigma_1^2 + \sigma_2^2)/2}$.

## MID-CIRCUIT MEASUREMENT

A bias magnetic field is applied during the Ramsey sequence, our simple quantum circuit, to lift the degeneracy of the Zeeman sublevels and confine the atom within the $m_F = 0$ subspace. The fluorescence measurement operates under a bias field of 5 G that is aligned with the propagation direction of the fluorescence probe beams, which allows for simultaneous one-dimensional sub-Doppler cooling during the measurement. We note that this field setting is different than for the fluorescence measurement characterized in Fig. 2 in the main text, for which the applied field is near zero. It is possible that the higher magnetic field setting used in this two-atom experiment increases the overall infidelity of measurement. However, this increased infidelity does not affect the main focus of the two-atom experiment, which is the characterization of additional decoherence on atom B owing to the mid-circuit measurement of atom A.

For the transmission measurements, the field orientation is rotated after state preparation to be aligned with the cavity axis, and the field amplitude is reduced to 2 G. This allows the atoms to be pumped into the stretched state by circularly-polarized transmission probe light during measurement. The microwave field driving the $\pi/2$ pulses has a Rabi frequency of $2\pi \times 2.1$ kHz and $2\pi \times 4.8$ kHz for the fluorescence and transmission measurements, respectively. This difference is due to field projection along different quantization axes.

To quantify the decoherence of the out-of-cavity atom induced by the local probe light, which is on for $2\tau$, and the local repump light, which is on for $\tau_{\rm rp}$, we measure the normalized Ramsey contrast $\tilde{\mathcal{C}}$ of atom B after measuring atom A with various $\tau$ and $\tau_{\rm rp}$ larger than the optimal value, as shown in Fig. S2. The measured results are fitted by a function

$$\tilde{\mathcal{C}}(\tau, \tau_{\rm rp}) = \exp\left[-(\lambda_1 \tau + \lambda_2 \tau_{\rm rp})\right], \tag{S1}$$

where $\lambda_1$ and $\lambda_2$ describe decoherence rates caused by the probe and repump light, respectively. This method gives a lower bound of $\tilde{\mathcal{C}} > 97.4\%$ with 84% confidence level for fluorescence detection with $(\tau, \tau_{\rm rp}) = (25\,\mu\text{s}, 5\,\mu\text{s})$ and atom distance $d = 34.5\,\mu$m, as well as $\tilde{\mathcal{C}} > 97.0\%$ for transmission detection with $(\tau, \tau_{\rm rp}) = (50\,\mu\text{s}, 5\,\mu\text{s})$ and atom distance $d = 46.0\,\mu$m—in both cases well away from the probe beam waist.

Let us assume that decoherence of atom B owing to the measurement on atom A is dominantly caused by atom B's direct exposure to probe light (i.e. not the secondary exposure to light scattered by atom A), and that a single scattered photon completely decoheres atom B. We can then estimate the decoherence rate $\lambda_1 = \mathcal{R} e^{-d^2/2w^2}$ where $\mathcal{R}$ is the scattering rate from an $F = 2$ atom at the location of maximum intensity of the probe beam ($d = 0$), and $w$ is the $1/e^2$ intensity probe beam waist radius. Values of $\mathcal{R}$ are determined already by the cavity emission observed when measuring single tweezer-trapped atoms; for the data of Fig. 4(c) (main text), we take these as $\mathcal{R} = 4.3\,\mu\text{s}^{-1}$ ($2.3\,\mu\text{s}^{-1}$) for fluorescence (transmission) measurements. In the case of fluorescence probing, the beam waists of the two counter-propagating probe beams differ: The downward-going beam (focused by the high-NA lens) has a beam waist around 3.3 $\mu$m, while the upward-going beam has a beam waist around 13 $\mu$m. For simplicity, for the above estimate, we simply use $w = 13\,\mu$m. In the case of transmission probing, we set $w = w_0$, matching the cavity mode waist. The reductions in normalized contrast predicted by this treatment are shown as dashed (fluorescence) and dotted (transmission) lines in Fig. 4(c).

## SPAM ERROR ANALYSIS

In Figs. 2 and 3 and Table 1, the reported infidelity on each state is the probability of the measurement outcome falling outside of the correct quadrant, calculated directly from the observed SPAM error over many experimental repetitions, and based on Bayesian probability theory.

Here, we describe how we distinguish state preparation error from measurement error. We focus our discussion on fluorescence detection. We describe a tweezed atom in the $F = 2$ manifold as the bright state, and the other tweezer state possibilities (empty tweezer, or tweezer with an atom in the $F = 1$ manifold) as dark states.

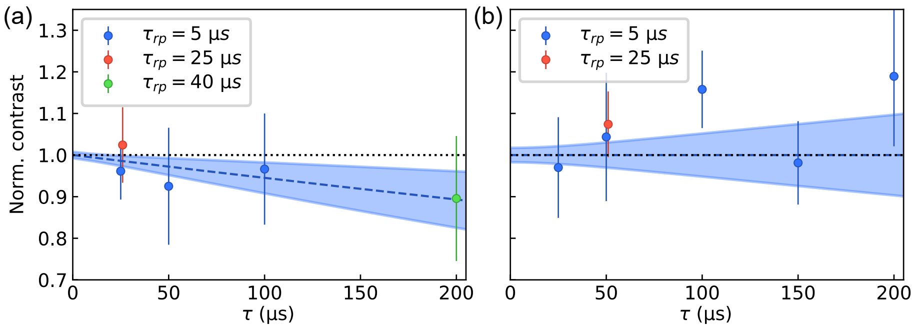


Figure S2. Normalized Ramsey contrast measured for atom B with various probe interval $\tau$ and repump time $\tau_{\mathrm{rp}}$ for atom A measurement. (a) Fluorescence measurement at a distance of $d = 34.5\,\mu$m. (b) Transmission measurement at a distance of $d = 46.0\,\mu$m. The blue dashed line indicates the fitted decoherence with $\tau_{\mathrm{rp}} = 5\,\mu$s, while the blue shaded area indicates the uncertainty of the fit.

State measurement error is the sum of single interval measurement (SIM) errors in each interval: $\epsilon_{F=2} = P^-$; $\epsilon_{F=1} = P^+ + P^-$; $\epsilon_{\mathrm{empty}} = 2P^+$. Here we define positive (negative) SIM errors $P^+(P^-)$ as the probability of having a first-interval photon count above (below) the bimodal threshold for a dark (bright) state atom. We set the threshold between 0 and 1 photons (which we denote as $n_{\mathrm{th}} = 0$) for $\tau \leq 15\,\mu$s and between 1 and 2 photons ($n_{\mathrm{th}} = 1$) for $\tau > 15\,\mu$s, so that $\max(P^+, P^-)$ is minimized.

The dark state photon counts follow a Poisson process of rate $R_{\mathrm{dark}} \simeq 0.4$ ms$^{-1}$(the dark count rate of the SPCM). Using the cumulative distribution function (CDF) of a Poisson distribution $Q(n_{\mathrm{th}}, \lambda) = e^{-\lambda} \sum_{m=0}^{n_{\mathrm{th}}} \frac{(\lambda)^m}{m!}$, we can write the positive SIM error as

$$P^+ = 1 - Q(n_{\mathrm{th}}, R_{\mathrm{dark}}\tau) \tag{S2}$$

The bright state photon count deviates from the Poisson distribution in two ways. First, Zeeman sampling and spatial sampling of $g$ randomize the scattering rate $\tilde{R}$, broadening the observed photon-count distribution above the Poisson limit by a Fano factor $\mathcal{F}$ observed to be 1.7 (2.2) for fluorescence (transmission) detection. Second, an $F = 2$ atom can either off-resonantly depump into the $F = 1$ manifold or be heated out of the tweezer trap mid-interval, resulting in a randomized fluorescence time $\tilde{t}$ with average lifetime $T$. A state-jump error occurs if the SPCM has not yet counted an above-threshold number of photons before the atom goes dark. The Poissonian CDF $\tilde{P}^-(\tilde{R}, \tilde{t}) = Q\left(n_{\mathrm{th}}, \tilde{R}\,\tilde{t}\right)$ also becomes a random variable, and we calculate the negative SIM error as its expectation value:

$$P^- = \mathbb{E}\left(\tilde{P}^-(\tilde{R}, \tilde{t})\right) = \int_0^\tau \rho_t(\tilde{t})\mathrm{d}\tilde{t} \int_0^\infty \rho_R(\tilde{R})\mathrm{d}\tilde{R}\; Q\left(n_{\mathrm{th}}, \tilde{R}\,\tilde{t}\right), \tag{S3}$$

where $\rho_R(\tilde{R}) \propto \mathrm{Exp}\left(-\frac{(\tilde{R}-R_{\mathrm{max}})^2}{2(\mathcal{F}-1)\tilde{R}_{\mathrm{max}}}\right)$ and $\rho_t(\tilde{t}) = \frac{1}{T}e^{-\tilde{t}/T} + e^{-\tau/T}\delta(\tilde{t} - \tau)$. As $\tau \to \infty$, while random sampling only slows down the speed at which $P^-$ asymptotes to 0, state-jump error causes $P^-$ to reach a mininum of $P^-_{\mathrm{sj}} = (1 + 2R_{\mathrm{max}}T)/(1 + R_{\mathrm{max}}T)^2 = 0.2\%$, where $T = 1.6$ ms is the measured bright state lifetime at $\varDelta_{\mathrm{pc}} = 2\pi \times (-10)$ MHz. This is lower than the measured $F = 2$ infidelity in the long probe limit ($\sim 0.5\%$) as shown Fig. 2(d). We take the remaining unaccounted error of 0.3% to be state preparation infidelity. For this setting, therefore, the state preparation error and measurement error are roughly equal in magnitude, as stated in the main text. By fixing the values above for $R_{\mathrm{dark}}$, $\mathcal{F}$, $T$ and the state preparation error, we obtain the predicted SPAM infidelities plotted as lines in Fig. 2(d).

For a larger detuning $\varDelta_{\mathrm{pc}} = 2\pi \times (-20)$ MHz, we increase the fluorescence beam intensity by roughly a factor of 4 to reach the same cavity scattering rate $R_{\mathrm{high}}$. At this intensity, we observe a shorter state lifetime of $T \simeq 0.4$ ms, corresponding to a state-jump error of $P^-_{\mathrm{sj}} \simeq 0.8\%$ and thus increasing the observed infidelity in the long probe limit to 1.1%.

A similar analysis can be carried out for transmission detection, where depump error will cause $P^-$ to increase with probe time at long probe times, as indicated by the lines showing the predicted SPAM infidelities in Fig. 3(d).

* These authors contributed equally to this work.
† dmsk@berkeley.edu

[S1] N. Schlosser, G. Reymond, I. Protsenko, and P. Grangier, Sub-Poissonian Loading of Single Atoms in a Microscopic Dipole Trap, Nature **411**, 1024 (2001).
[S2] E. Deist, J. A. Gerber, Y.-H. Lu, J. Zeiher, and D. M. Stamper-Kurn, Superresolution microscopy of optical fields using tweezer-trapped single atoms, Phys. Rev. Lett. **128**, 083201 (2022).
[S3] C. Tuchendler, A. M. Lance, A. Browaeys, Y. R. P. Sortais, and P. Grangier, Energy distribution and cooling of a single atom in an optical tweezer, Phys. Rev. A **78**, 033425 (2008), arXiv:0805.3510.
[S4] A. M. Kaufman, B. J. Lester, and C. A. Regal, Cooling a Single Atom in an Optical Tweezer to Its Quantum Ground State, Phys. Rev. X **2**, 041014 (2012).
[S5] J. A. Gerber, *Cavity Quantum Electrodynamics with a Locally Addressable Quantum Gas*, Ph.D. thesis, University of California Berkeley (2020).
[S6] J. R. Johansson, P. D. Nation, and F. Nori, QuTiP 2: A Python framework for the dynamics of open quantum systems, Comput. Phys. Commun. **184**, 1234 (2013).
[S7] J. Bochmann, M. Mücke, C. Guhl, S. Ritter, G. Rempe, and D. L. Moehring, Lossless State Detection of Single Neutral Atoms, Phys. Rev. Lett. **104**, 203601 (2010).
[S8] K. A. Ashman, C. M. Bird, and S. E. Zepf, Detecting bimodality in astronomical datasets, Astron. J. **108**, 2348 (1994).
